# Supplementary material for: Bridging constrained random-phase approximation and linear response theory for computing Hubbard parameters
Source: arXiv:2505.03698 ancillary file (2025-12-23)
Supplement: Supplementary file 1 [file supplementary.pdf]

# Supplemental material to the manuscript "Bridging constrained random-phase approximation and linear response theory for computing Hubbard parameters"


Alberto Carta,[1, *] Iurii Timrov,[2, †] Sophie Beck,[3] and Claude Ederer[1, ‡]

[1] *Materials Theory, ETH Zürich, Wolfgang-Pauli-Strasse 27, 8093 Zürich, Switzerland*
[2] *PSI Center for Scientific Computing, Theory, and Data, 5232 Villigen PSI, Switzerland*
[3] *Center for Computational Quantum Physics, Flatiron Institute, 162 5th Avenue, New York, NY 10010, USA*



(Dated: May 6, 2025)


In Sec. I of this supplemental material we present full details of the mathematical relationship between the Hubbard parameters computed within linear response theory (LRT) and the constrained random-phase approximation (cRPA). In addition, Sec. II provides details of our implementation for calculating Hubbard parameters using density functional perturbation theory with Wannier projectors, while Sec. III contains the computational details of the calculations presented in the main text.

Furthermore, Sec. I is structured as follows. In Sec. I A, we first summarize the results presented by Himmetoglu *et al.* [1], introducing the susceptibility matrices in a generalized LRT framework, which later enter the expressions for the interaction parameters. We always refer to this more general framework as *generalized LRT*, while the commonly implemented "standard" way of computing the Hubbard parameters, as described for instance in the original paper of Cococcioni and de Gironcoli [2], will be referred as *coarse-grained LRT*. In Sec. I B, we consider the restriction of the susceptibility matrices to the interacting subspace $\mathcal{D}$, a necessary step to later compare the two methods. RPA and cRPA are discussed in Sec. I C, and in Sec. I D, we demonstrate under which approximations generalized LRT and cRPA can be regarded as equivalent. In Sec. I E, we summarize the concept of *"coarse graining"* of the susceptibility matrices, following again Himmetoglu *et al.* [1]. Finally, our main result is presented in Sec. I F, where we explicitly show how the expressions for the Hubbard parameter obtained in the two methods are related.

## I. RELATION BETWEEN THE HUBBARD PARAMETER CALCULATED USING LINEAR RESPONSE THEORY AND THE PARTIALLY SCREENED INTERACTION OBTAINED WITHIN CONSTRAINED RANDOM PHASE APPROXIMATION

### A. Generalized linear response theory

As discussed by Himmetoglu et al. [1], the LRT calculation of the $U$ parameter can be generalized by considering an external perturbation that can be non-local and orbitally off-diagonal:

$$\Delta V_{\text{ext}} = \sum_{IJ} \sum_{ij} \lambda_{ij}^{IJ} \left|\phi_i^I\right\rangle \left\langle\phi_j^J\right| := \sum_{ij}^{IJ} \lambda_{ij}^{IJ} \left|\phi_i^I\right\rangle \left\langle\phi_j^J\right| \quad . \tag{1}$$

In this expression, $\lambda_{ij}^{IJ}$ represents the perturbation to the on-site potential within a localized basis $\left|\phi_i^I\right\rangle$, where the index $I$ indexes both the site (atom) and shell (e.g., $s$, $p$, $d$, $f$), while the $i$ index denotes the orbitals within the shell. To keep the presentation compact, we always indicate the summation over the site/shell indices on top of the summation symbol, as defined in Eq. (1), while the orbital indices are placed below the summation symbol as usual.

The change of the Kohn-Sham potential (to linear order in the perturbation), $\Delta V_{\text{scf}}$, is then given by the sum of the external perturbation $\Delta V_{\text{ext}}$ and the induced changes in both the Hartree, $\Delta V_H$, and exchange-correlation, $\Delta V_{xc}$, potentials:

$$\Delta V_{\text{scf}} = \Delta V_{\text{ext}} + \Delta V_H + \Delta V_{xc} \quad , \tag{2}$$


*Electronic address: alberto.carta@mat.ethz.ch
†Electronic address: iurii.timrov@psi.ch
‡Electronic address: edererc@ethz.ch

with:

$$\Delta V_H(\mathbf{r}) = \int \frac{\Delta\rho(\mathbf{r}')}{|\mathbf{r}-\mathbf{r}'|} d\mathbf{r}'$$
$$\Delta V_{xc}(\mathbf{r}) = \int \frac{\delta V_{xc}(\mathbf{r})}{\delta\rho(\mathbf{r}')} \Delta\rho(\mathbf{r}') d\mathbf{r}' \quad , \tag{3}$$

and the variation in the density at position $\mathbf{r}$ is denoted by $\Delta\rho(\mathbf{r})$. The first order change to the Kohn-Sham orbital $|\psi_n\rangle$ with eigenvalue $\epsilon_n$ is given by:

$$|\Delta\psi_n\rangle = \sum_{m\neq n} \frac{\langle\psi_m|\Delta V_{scf}|\psi_n\rangle}{\epsilon_n - \epsilon_m} |\psi_m\rangle \quad . \tag{4}$$

We note that $m$ and $n$ should be viewed as compound indices indicating k-point, band, and spin character. Similarly, $i$ and $j$ in Eq. (1) indicate both orbital and spin character. However, in the following, we always implicitly consider the spin degenerate case.

We assume that the local orbitals $|\phi_i^I\rangle$ form a complete and orthonormal basis set for the Kohn-Sham states. This is certainly true if the $|\phi_i^I\rangle$ are constructed as Wannier functions from the Kohn-Sham Bloch states within the relevant energy window. The corresponding density matrix $n_{ij}^{IJ}$ is given by:

$$n_{ij}^{IJ} = \sum_n f_n \langle\phi_i^I|\psi_n\rangle\langle\psi_n|\phi_j^J\rangle, \tag{5}$$

where $f_n$ is the occupation of the Kohn-Sham state $|\psi_n\rangle$. The variation of the density matrix due to the perturbation reads:

$$\Delta n_{ij}^{IJ} = \sum_n f_n \left[\langle\psi_n|\phi_j^J\rangle\langle\phi_i^I|\Delta\psi_n\rangle + \langle\Delta\psi_n|\phi_j^J\rangle\langle\phi_i^I|\psi_n\rangle\right]$$
$$= \sum_{n,m} \frac{f_n - f_m}{\epsilon_n - \epsilon_m} \langle\phi_i^I|\psi_m\rangle\langle\psi_m|\Delta V_{scf}|\psi_n\rangle\langle\psi_n|\phi_j^J\rangle \quad , \tag{6}$$

where we assume that we can neglect any contribution related to variations of the occupations $f_n$ caused by the shift of the Kohn-Sham states. This approximation becomes exact in the limit of an infinite crystal with a non-periodic perturbation localized on a single site, as pointed out by Baroni *et al.* [3]. Recasting Eq. (6) in terms of only matrix elements in the localized basis one can write [1]:

$$\Delta n_{ij}^{IJ} = \sum_{mn} \sum_{kl}^{KL} \frac{f_n - f_m}{\epsilon_n - \epsilon_m} \langle\phi_i^I|\psi_m\rangle\langle\psi_m|\phi_k^K\rangle\langle\phi_k^K|\Delta V_{\rm scf}|\phi_l^L\rangle\langle\phi_l^L|\psi_n\rangle\langle\psi_n|\phi_j^J\rangle \tag{7}$$

One can then define the "bare" $(\chi_0)$ and "full" $(\chi)$ susceptibility matrices from the equations [1]:

$$\Delta n_{ij}^{IJ} = \sum_{kl}^{KL} (\chi_0)_{ijlk}^{IJLK} \langle\phi_k^K|\Delta V_{\rm scf}|\phi_l^L\rangle \tag{8}$$

and

$$\Delta n_{ij}^{IJ} = \sum_{kl}^{KL} \chi_{ijlk}^{IJLK} \langle\phi_k^K|\Delta V_{\rm ext}|\phi_l^L\rangle = \sum_{kl}^{KL} \chi_{ijlk}^{IJLK} \lambda_{kl}^{KL} \quad . \tag{9}$$

By comparing Eq. (7) and Eq. (8), one obtains the expression for the bare susceptibility:

$$(\chi_0)_{ijlk}^{IJLK} = \sum_{mn} \frac{f_n - f_m}{\epsilon_n - \epsilon_m} \langle\phi_i^I|\psi_m\rangle\langle\psi_n|\phi_j^J\rangle\langle\phi_l^L|\psi_n\rangle\langle\psi_m|\phi_k^K\rangle \quad . \tag{10}$$

As shown in [1], by explicitly writing out the expression for $\Delta V_{\rm scf}$, the full and bare susceptibilities can be related in terms of a Dyson equaton of the form:

$$\chi_{ijlk}^{IJLK} = (\chi_0)_{ijlk}^{IJLK} + \sum_{opqs}^{OPQS} (\chi_0)_{ijpo}^{IJPO} \mathcal{I}_{opqs}^{OPQS} \chi_{sqlk}^{SQLK} \quad , \tag{11}$$

where the matrix elements of the kernel $\mathcal{I}_{opsr}^{OPSR}$ are given by:

$$\mathcal{I}_{opsr}^{OPSR} = \int\int \phi_o^O(\mathbf{r})^* \phi_p^P(\mathbf{r}) \left[ V(\mathbf{r},\mathbf{r}') + \frac{\delta V_{xc}(\mathbf{r})}{\delta\rho(\mathbf{r}')} \right] \phi_s^S(\mathbf{r}')^* \phi_r^R(\mathbf{r}')\, d\mathbf{r}\, d\mathbf{r}' \tag{12}$$

with $\phi_o^O(\mathbf{r}) = \langle \mathbf{r} | \phi_o^O \rangle$ and the bare Coulomb interaction $V(\mathbf{r},\mathbf{r}') = 1/|\mathbf{r}-\mathbf{r}'|$.

Eq. (11) can also be written in matrix notation:

$$\begin{aligned} \chi &= \chi_0 + \chi_0 \mathcal{I} \chi \\ &= \chi_0 + \chi_0 \mathcal{I} \chi_0 + \chi_0 \mathcal{I} \chi_0 \mathcal{I} \chi_0 + ... \\ &= \chi_0 + \chi_0 \mathcal{W} \chi_0 \quad , \end{aligned} \tag{13}$$

where we have defined the fully screened interaction kernel, $\mathcal{W}$, which can be expressed as a geometric series of the bare kernel $\mathcal{I} = V + \delta V_{xc}/\delta\rho$ and the bare susceptibility $\chi_0$:

$$\mathcal{W} = \mathcal{I} + \mathcal{I}\chi_0\mathcal{I} + \mathcal{I}\chi_0\mathcal{I}\chi_0\mathcal{I} + ... \tag{14}$$

### B. Generalized LRT restricted to the target subspace

In this section, we divide the Hilbert space into a “target” subspace $\mathcal{D}$, and a “ rest” subspace, $\mathcal{S}$, according to $\mathcal{H} = \mathcal{D} \bigoplus \mathcal{S}$. Furthermore, in the following we always assume that the target space corresponds to an isolated set of bands, and apply this to the framework of generalized LRT. This division of the Hilbert space is also central to the formulation of cRPA (discussed in Sec. I C) and the specific case corresponding to isolated sets of bands will enable a direct connection between the physical quantities computed within the two approaches in Sec. I F.

If the two subspaces $\mathcal{D}$ and $\mathcal{S}$ correspond to isolated sets of bands, then both the Bloch states, $|\psi_n\rangle$, and the local basis orbitals, $|\phi_i^I\rangle$, can be uniquely assigned to either $\mathcal{D}$ or $\mathcal{S}$. We can then easily identify the components of the bare susceptibility matrix that correspond only to the target subspace:

$$\begin{aligned} &X_{ijlk}^{IJLK} = \chi_{ijlk}^{IJLK} \\ &(X_0)_{ijlk}^{IJLK} = (\chi_0)_{ijlk}^{IJLK} \\ &\text{with } \{I,J,K,L,i,j,k,l\} \in \mathcal{D} \quad , \end{aligned} \tag{15}$$

i.e., we indicate with the symbol $X$ the susceptibility components that correspond exclusively to $\mathcal{D}$.

For the corresponding bare susceptibility, one can write:

$$(X_0)_{ijlk}^{IJLK} = \sum_{m\in\mathcal{D}} \sum_{n\in\mathcal{D}} \frac{f_n - f_m}{\epsilon_n - \epsilon_m} \langle \phi_i^I | \psi_m \rangle \langle \psi_n | \phi_j^J \rangle \langle \phi_l^L | \psi_n \rangle \langle \psi_m | \phi_k^K \rangle \quad , \tag{16}$$

i.e., one can simply restrict the sums in the definition of $X_0$ to $m, n \in \mathcal{D}$. In order to obtain a similar expression for $X$, we turn to Eq. (13) and restrict all indices outside of the sum to $\mathcal{D}$:

$$\begin{aligned} X_{ijlk}^{IJLK} &= (X_0)_{ijlk}^{IJLK} + \sum_{opqz}^{OPQZ} (\chi_0)_{ijop}^{IJOP} \mathcal{I}_{pozq}^{POZQ} (\chi)_{qzlk}^{QZLK} \\ &= (X_0)_{ijlk}^{IJLK} + \sum_{opqz}^{OPQZ} (\chi_0)_{ijop}^{IJOP} \mathcal{W}_{pozq}^{POZQ} (\chi_0)_{qzlk}^{QZLK} \\ &\text{with } \{I,J,K,L,i,j,k,l\} \in \mathcal{D} \text{ and } \{O,P,Q,Z,o,p,q,z\} \in \mathcal{H} \quad . \end{aligned} \tag{17}$$

Examining the full expression of the bare susceptibility in Eq. (10) and using $\mathcal{H} = \mathcal{D} \bigoplus \mathcal{S}$, we observe that for any non-zero matrix element between $|\phi_i^I\rangle$ and $|\phi_j^J\rangle$ (with $|\phi_i^I\rangle, |\phi_j^J\rangle \in \mathcal{D}$), the states $|\psi_n\rangle$ and $|\psi_m\rangle$ must also belong to $\mathcal{D}$. Consequently, $(\chi_0)_{ijop}^{IJOP} = 0$ if either $|\phi_o^O\rangle$ or $|\phi_p^P\rangle$ are not in $\mathcal{D}$. However, it is important to note that generally, $(\chi_0)_{iopj}^{IOPJ} \neq 0$, due to the different order of indices, as this order implies selecting only one state $|\psi_n\rangle \in \mathcal{D}$ in the sum of Eq. (10). These considerations allow us to rewrite equation Eq. (17) using only $X_0$ and considering all indices in the sum only within $\mathcal{D}$:

$$\begin{aligned} X_{ijlk}^{IJLK} &= (X_0)_{ijlk}^{IJLK} + \sum_{opqz}^{OPQZ} (X_0)_{ijop}^{IJOP} \mathcal{W}_{pozq}^{POZQ} (X_0)_{qzlk}^{QZLK} \\ &\text{with } \{O,P,Q,Z,o,p,q,z\} \in \mathcal{D} \quad . \end{aligned} \tag{18}$$

Crucially, Eq. (18) relates the quantities $X$, $X_0$, and $\mathcal{W}$ that are entirely restricted to the interacting subspace $\mathcal{D}$. In Sec. I D we will show that closely related quantities are computed within the cRPA framework.

### C. Introducing the (constrained) random phase approximation

In this section, we first introduce the random-phase approximation (RPA) and relate the static components of the bare RPA susceptibility and the fully screened interaction to the corresponding quantities within generalized LRT. Then, we summarize the main features of the constrained random phase approximation (cRPA) as reported in the literature.

Within RPA, the fully screened Coulomb interaction $W$ can be expressed as an infinite series in the Coulomb interaction $V(\mathbf{r},\mathbf{r}')$ [1]:

$$\begin{aligned} W &= V + V\chi_0 V + V\chi_0 V\chi_0 V + \dots \\ &= \left[1 - V\chi_0\right]^{-1} V \quad , \end{aligned} \tag{19}$$

where $\chi_0(\omega,\mathbf{r},\mathbf{r}')$ is the bare RPA susceptibility, which can be expressed as:

$$\chi_0(\omega,\mathbf{r},\mathbf{r}') = \sum_{m,n} \frac{f_n - f_m}{\omega + \epsilon_n - \epsilon_m} \langle \mathbf{r}|\psi_m\rangle\langle\psi_n|\mathbf{r}\rangle\langle\mathbf{r}'|\psi_n\rangle\langle\psi_m|\mathbf{r}'\rangle \quad . \tag{20}$$

We note that the RPA generally considers the response to a space- and time-dependent perturbation and thus the corresponding susceptibility is frequency-dependent and describes the change in density at point $\mathbf{r}$, due to a variation of the external potential at point $\mathbf{r}'$. However, it is easy to see that the static component $\chi_0(\omega = 0,\mathbf{r},\mathbf{r}')$ of Eq. (20) is completely equivalent to the generalized bare susceptibility defined in Eq. (10) if transformed to the local orbital basis. This can be seen by using $|\psi_m\rangle = \sum_i^I |\phi_i^I\rangle\langle\phi_i^I|\psi_m\rangle$ in Eq. (20), which leads to:

$$\chi_0(0,\mathbf{r},\mathbf{r}') = \sum_{ijkl}^{IJKL} \langle\mathbf{r}|\phi_i^I\rangle\langle\phi_j^J|\mathbf{r}\rangle\langle\mathbf{r}'|\phi_l^L\rangle\langle\phi_k^K|\mathbf{r}'\rangle \underbrace{\sum_{m,n}\frac{f_n - f_m}{\epsilon_n - \epsilon_m}\langle\phi_i^I|\psi_m\rangle\langle\psi_n|\phi_j^J\rangle\langle\phi_l^L|\psi_n\rangle\langle\psi_m|\phi_k^K\rangle}_{(\chi_0)_{ijlk}^{IJLK}} \quad . \tag{21}$$

Consequently, we use the same symbol $\chi_0$ to indicate both the bare RPA and the bare generalized susceptibility. [2]

We also note that, by comparing Eq. (14) with the first line in Eq. (19), one can further identify the fully screened interaction $\mathcal{W}$ with the fully screened RPA interaction $W$, if one neglects the exchange-correlation part of the interaction kernel $\mathcal{I}$ or, equivalently, assumes $\mathcal{I} \approx V$. This will become important in Sec. I F, where we derive the relation between the screened interaction parameters obtained in LRT and cRPA.

The *constrained* RPA approach [5, 6] is based on the separation of the Hilbert space into target and rest subspaces, $\mathcal{H} = \mathcal{D} \bigoplus \mathcal{S}$, as introduced in Sec. I B, and the corresponding separation of the bare susceptibility in two components:

$$\chi_0 = \chi_0^{\mathcal{D}} + \chi_0^{\mathcal{R}} \quad . \tag{22}$$

Here, $\chi_0^{\mathcal{D}}$ contains the subset of two-particle excitations happening completely within the $\mathcal{D}$ subspace and thus reads:

$$\chi_0^{\mathcal{D}}(\omega,\mathbf{r},\mathbf{r}') = \sum_{m,n\in\mathcal{D}} \frac{f_n - f_m}{\omega + \epsilon_n - \epsilon_m} \langle \mathbf{r}|\psi_m\rangle\langle\psi_n|\mathbf{r}\rangle\langle\mathbf{r}'|\psi_n\rangle\langle\psi_m|\mathbf{r}'\rangle \quad . \tag{23}$$

The remaining part of the susceptibility, $\chi_0^{\mathcal{R}}$, encodes all other two-particle excitations, i.e., the superscript $\mathcal{R}$ denotes excitations happening completely within the $\mathcal{S}$ subspace as well as the ones happening between $\mathcal{S}$ and $\mathcal{D}$. Again, we note that in analogy to Eq. (21), the static component ($\omega = 0$) of $\chi_0^{\mathcal{D}}$ is equivalent to the generalized bare susceptibility restricted to the target subspace, i.e., to the quantity $X_0$ defined in Eq. (16).

---

[1] All quantities expressed in matrix notation in Eq. (19) are functions of two spatial coordinates and the corresponding "matrix product" implies integration over the joint coordinate.

[2] Note that $\chi_0(\omega,\mathbf{r},\mathbf{r}')$ can be viewed as "bi-local" component, $\chi_0(\omega,\mathbf{r},\mathbf{r}') := L_0(\omega,\mathbf{r},\mathbf{r},\mathbf{r}',\mathbf{r}')$, of a more general response function $L_0(\omega,\mathbf{r},\mathbf{r}'',\mathbf{r}',\mathbf{r}''')$, which depends on four spatial coordinates (see, e.g., [4]). Since the Coulomb interaction, $V(\mathbf{r},\mathbf{r}') = 1/|\mathbf{r}-\mathbf{r}'|$, is also bi-local, only $\chi_0(\omega,\mathbf{r},\mathbf{r}')$ is required to compute the screening. However, in the local orbital basis, the four-component form reappears.

One can now define the *partially screened* Coulomb interaction [5, 6]:

$$W^{\mathcal{R}} = \left[1 - V\chi_0^{\mathcal{R}}\right]^{-1} V \quad , \tag{24}$$

which only includes the screening represented by $\chi_0^{\mathcal{R}}$. The matrix elements of $W^{\mathcal{R}}$ in a suitably chosen localized basis spanning the $\mathcal{D}$ subspace then define the partially screened interaction parameters within $\mathcal{D}$. In the context of DFT+DMFT or DFT+$U$ calculations, one typically only considers the static component:

$$(W^{\mathcal{R}})_{opsr}^{OPSR} = \iint \phi_o^O(\mathbf{r})^* \phi_p^P(\mathbf{r}) W^{\mathcal{R}}(\omega = 0, \mathbf{r}, \mathbf{r}') \phi_s^S(\mathbf{r}')^* \phi_r^R(\mathbf{r}') \, d\mathbf{r} \, d\mathbf{r}' \quad . \tag{25}$$

The fully screened interaction from Eq. (19) is then obtained by combining Eq. (24) with Eq. (19) and Eq. (22):

$$\begin{aligned} W &= \left[1 - V\chi_0^{\mathcal{D}} - V\chi_0^{\mathcal{R}}\right]^{-1} V \\ &= \left[(1 - V\chi_0^{\mathcal{R}})(1 - (1 - V\chi_0^{\mathcal{R}})^{-1} V\chi_0^{\mathcal{D}})\right]^{-1} V \\ &= \left[1 - (1 - V\chi_0^{\mathcal{R}})^{-1} V\chi_0^{\mathcal{D}})\right]^{-1} (1 - V\chi_0^{\mathcal{R}})^{-1} V \\ &= \left[1 - W^{\mathcal{R}}\chi_0^{\mathcal{D}}\right]^{-1} W^{\mathcal{R}} \quad . \end{aligned} \tag{26}$$

We can also expand the geometric series in the last line of Eq. (26) to obtain:

$$W = W^{\mathcal{R}} + W^{\mathcal{R}}\chi_0^{\mathcal{D}}W^{\mathcal{R}} + W^{\mathcal{R}}\chi_0^{\mathcal{D}}W^{\mathcal{R}}\chi_0^{\mathcal{D}}W^{\mathcal{R}} + \ldots \tag{27}$$

The screening in cRPA can thus be viewed as a two-step process. First, the screening involving the $\mathcal{S}$ subspace is applied to obtain the partially screened interaction $W^{\mathcal{R}}$ (Eq. (24)), which can be used as effective interaction in a model-like description involving only the $\mathcal{D}$ subspace. Then, in a second step, the screening within $\mathcal{D}$ results in the fully screened interaction $W$ (Eq. (26)).

### D. Relation between generalized LRT and cRPA

Next, we show how the interaction tensor computed in cRPA can be related to the interaction from the generalized LRT method. Together with Sec. I F, where we relate cRPA to the coarse gained LRT, this constitutes the main analytical result of our work.

From Eq. (27) we can deduce a natural definition of the "full" cRPA susceptibility $\chi^{\mathcal{D}}$, written as:

$$\begin{aligned} \chi^{\mathcal{D}} &= \chi_0^{\mathcal{D}} + \chi_0^{\mathcal{D}}W^{\mathcal{R}}\chi_0^{\mathcal{D}} + \chi_0^{\mathcal{D}}W^{\mathcal{R}}\chi_0^{\mathcal{D}}W^{\mathcal{R}}\chi_0^{\mathcal{D}} + \ldots \\ \chi^{\mathcal{D}} &= \chi_0^{\mathcal{D}} + \chi_0^{\mathcal{D}}W^{\mathcal{R}}\chi^{\mathcal{D}} \quad . \end{aligned} \tag{28}$$

By formally inverting the Dyson equation, Eq. (28), we obtain:

$$W^{\mathcal{R}} = (\chi_0^{\mathcal{D}})^{-1} - (\chi^{\mathcal{D}})^{-1} \quad . \tag{29}$$

To highlight the equivalence between cRPA and the generalized LRT restricted to the target subspace, we can use the already established equivalence between $\chi_0^{\mathcal{D}}$ and $X_0$ and, as noted in Sec. I C, identify $W$ from Eq. (27) and Eq. (19) with $\mathcal{W}$ from Eq. (14) if we neglect the exchange-correlation kernel or assume $\mathcal{I} \simeq V$. This transforms Eq. (27) into:

$$\mathcal{W} \simeq W^{\mathcal{R}} + W^{\mathcal{R}}X_0W^{\mathcal{R}} + W^{\mathcal{R}}X_0W^{\mathcal{R}}X_0W^{\mathcal{R}} + \ldots \quad , \tag{30}$$

which can now be read as a matrix equation with all matrix components corresponding to the local basis orbitals of the target subspace $\mathcal{D}$.

We can then substitute equation Eq. (30) into Eq. (18), resulting in:

$$\begin{aligned} X &= X_0 + X_0W^{\mathcal{R}}X_0 + X_0W^{\mathcal{R}}X_0W^{\mathcal{R}}X_0 + \ldots \\ X &= X_0 + X_0W^{\mathcal{R}}X \quad . \end{aligned} \tag{31}$$

Inverting the Dyson equation in the last line of Eq. (31) gives:

$$W^{\mathcal{R}} = X_0^{-1} - X^{-1} \quad . \tag{32}$$

This means that $\chi^{\mathcal{D}}$ is equivalent to the generalized suceptibility $X$, and the generalized linear response approach is equivalent to cRPA, provided that one neglects the exchange-correlation part $\delta V_{xc}(\mathbf{r})/\delta\rho(\mathbf{r}')$ in the definition of the kernel $\mathcal{I}$, Eq. (12).

### E. Definition of $U$ within the coarse-grained LRT approach

In this section, we describe how the commonly implemented version of the LRT method is obtained by "coarse graining" of the generalized susceptibility matrices introduced in Sec. I A. Thereby, we closely follow the presentation of Himmetoglu *et al.* [1].

In the LRT method introduced by Cococcioni and de Gironcoli [2], one considers only onsite ($I = J$) perturbations that are uniformly applied over all the orbitals of one atomic site $I$ (proportional to $\lambda^I$ times the projector on the target subspace). More explicitly this reads (see Eq. (1)):

$$\Delta V_{\text{ext}} = \sum_{ij}^{IJ} \lambda_{ij}^{IJ} \left|\phi_i^I\right\rangle \left\langle\phi_j^J\right| \rightarrow \sum_{i}^{I} \lambda^I \left|\phi_i^I\right\rangle \left\langle\phi_i^I\right| \quad . \tag{33}$$

The total on-site variation of the electronic occupation is then given by:

$$\begin{aligned} \Delta n^I &= \sum_i \Delta n_{ii}^{II} = \sum_i \sum_{kl}^{KL} \chi_{iilk}^{IILK} \lambda^K \delta_{kl} \delta^{KL} \\ &= \sum^{K} \lambda^K \sum_{ik} \chi_{iikk}^{IIKK} \quad . \end{aligned} \tag{34}$$

This motivates the definition of the "coarse-grained" susceptibilities:

$$\begin{aligned} \tilde{\chi}^{IJ} &= \sum_{ij} \chi_{iijj}^{IIJJ} \quad \text{and} \\ \tilde{\chi}_0{}^{IJ} &= \sum_{ij} (\chi_0)_{iijj}^{IIJJ} \quad . \end{aligned} \tag{35}$$

Importantly, we note that here the site indices $I$ and $J$, and the corresponding orbital indices $i$ and $j$, are restricted to a subset of the complete local basis set, referred to as the Hubbard manifold. In the following, we will always identify the Hubbard manifold with the target subspace $\mathcal{D}$ and assume that this subspace corresponds to an isolated set of bands, as discussed in the previous subsections. Thus, the general susceptibilites in the definition of $\tilde{\chi}$ and $\tilde{\chi}_0$ could also be replaced by $X$ and $X_0$.

The screened interaction tensor $U_{\text{LRT}}$ is defined from $\tilde{\chi}$ and $\tilde{\chi}_0$ as [2]:

$$U_{\text{LRT}} = (\tilde{\chi}_0)^{-1} - \tilde{\chi}^{-1} \quad , \tag{36}$$

which can also be written in a Dyson form similar to Eq. (11) and Eq. (28):

$$\tilde{\chi} = \tilde{\chi}_0 + \tilde{\chi}_0 U_{\text{LRT}} \tilde{\chi} \quad . \tag{37}$$

As shown in [1], by applying the definitions in Eq. (35) to Eq. (11) and comparing with Eq. (37), one can relate the coarse-grained screened interaction tensor, $U_{\text{LRT}}$, to the general interaction kernel $\mathcal{I}_{opqs}^{OPQS}$:

$$(U_{\text{LRT}})^{IJ} = \sum_{zt}^{ZT} \sum_{opqs}^{OPQS} (\tilde{\chi}_0^{-1})^{IZ} \left[ (\chi_0)_{zzpo}^{ZZPO} \mathcal{I}_{opqs}^{OPQS} \chi_{sqtt}^{SQTT} \right] (\tilde{\chi}^{-1})^{TJ} \tag{38}$$

Note that here, $\{I, J, Z, T, z, t\}$ are restricted to the target Hubbard manifold, while the indeces $\{O, P, Q, S, o, p, q, s\}$ run over the complete local basis set. As discussed by Himmetoglu [1] *et al.*, the screening of the bare kernel $\mathcal{I}$ operates via the summation over the unrestricted indices on the right hand side of Eq. (38).

In the next section, we apply an analogous procedure as detailed above to the susceptibility matrices restricted to the target subspace $\mathcal{D}$. This enables us to make explicit the relationship between $U_{\text{LRT}}$ and $U_{cRPA}$.

### F. Relation between coarse-grained LRT and cRPA

In spite of the similarity of the corresponding equations, $U_{\text{LRT}}$ from Eq. (36) and $W^{\mathcal{R}}$ from Eq. (29) and Eq. (32) are distinct quantities, as are $\chi^{\mathcal{D}}$ and $\tilde{\chi}$ as well as $\chi_0^{\mathcal{D}}$ and $\tilde{\chi}_0$. This is evident from the dimensionality of these quantities,

since $U_{\mathrm{LRT}}$, $\tilde{\chi}$, and $\tilde{\chi}_0$ are two component matrices, while $W^{\mathcal{R}}$, $\chi^{\mathcal{D}}$ and $\chi_0^{\mathcal{D}}$ are 4-index tensors. In the following, we show that, even though $\tilde{\chi}$ and $\tilde{\chi}_0$ are defined as averages over the components of $\chi^{\mathcal{D}}$ and $\chi_0^{\mathcal{D}}$ (or, equivalently, $X$ and $X_0$), $U_{\mathrm{LRT}}$ cannot be obtained as a similar simple average over the $W^{\mathcal{R}}$ matrix elements. Instead, additional screening processes are involved in $U_{\mathrm{LRT}}$ compared to $W^{\mathcal{R}}$.

We revisit the definition of $\tilde{\chi}$ and $\tilde{\chi}_0$ in terms of $X$ and $X_0$. Analogous to Eq. (35), we can write:

$$\begin{aligned}\tilde{\chi}^{IJ} &= \sum_{ij} \chi_{iijj}^{IIJJ} = \sum_{ij} X_{iijj}^{IIJJ} \quad , \\ \tilde{\chi}_0{}^{IJ} &= \sum_{ij} (\chi_0)_{iijj}^{IIJJ} = \sum_{ij} (X_0)_{iijj}^{IIJJ} \quad .\end{aligned} \tag{39}$$

Combining Eq. (37) and Eq. (31), using the definitions of $\tilde{\chi}$ and $\tilde{\chi}_0$ in Eq. (39) leads to:

$$\sum^{ZT} \tilde{\chi}_0{}^{IZ} (U_{LRT})^{ZT} \tilde{\chi}^{TR} = \sum_{ir} \sum_{opqs}^{OPQS} (X_0)_{iipo}^{IIPO} (W^{\mathcal{R}})_{opqs}^{OPQS} X_{sqrr}^{SQRR} \quad . \tag{40}$$

We can then obtain the matrix elements of $U_{\mathrm{LRT}}$ by multiplying Eq. (40) with $(\tilde{\chi}_0)^{-1}$ and $\tilde{\chi}^{-1}$ from the left and right, respectively. This leads to the following expression:

$$(U_{\mathrm{LRT}})^{IR} = \sum_{zt}^{ZT} \sum_{opqs}^{OPQS} (\tilde{\chi}_0^{-1})^{IZ} \left[ (X_0)_{zzpo}^{ZZPO} (W^{\mathcal{R}})_{opqs}^{OPQS} X_{sqtt}^{SQTT} \right] (\tilde{\chi}^{-1})^{TR} \quad . \tag{41}$$

By following Himmetoglu *et al.* [1], we can split the components of $X$ and $X_0$ into a bi-diagonal component and the rest, according to:

$$X_{ztss}^{ZTSS} = X_{ttss}^{TTSS} \delta^{TZ} \delta_{tz} + \bar{X}_{ztss}^{ZTSS} \quad , \tag{42}$$

where by definition $\bar{X}_{ttss}^{TTSS} = 0$. If we substitute this into Eq. (41) and simultaneously replace $(W^{\mathcal{R}})_{ppqq}^{PPQQ}$ with the corresponding orbital average $\langle\langle W^{\mathcal{R}} \rangle\rangle^{PPQQ}$, one finally obtains:

$$\begin{aligned}(U_{\mathrm{LRT}})^{IR} &= \langle\langle W^{\mathcal{R}} \rangle\rangle^{IIRR} \\ &+ \sum_{zt}^{ZT} \sum_{ops}^{OPS} (\tilde{\chi}_0^{-1})^{IZ} \left[ (\bar{X}_0)_{zzpo}^{ZZPO} (W^{\mathcal{R}})_{opss}^{OPSS} X_{sstt}^{SSTT} \right] (\tilde{\chi}^{-1})^{TR} \\ &+ \sum_{zt}^{ZT} \sum_{pqs}^{PQS} (\tilde{\chi}_0^{-1})^{IZ} \left[ (X_0)_{zzpp}^{ZZPP} (W^{\mathcal{R}})_{ppqs}^{PPQS} \bar{X}_{sqtt}^{SQTT} \right] (\tilde{\chi}^{-1})^{TR} \\ &+ \sum_{zt}^{ZT} \sum_{opqs}^{OPQS} (\tilde{\chi}_0^{-1})^{IZ} \left[ (\bar{X}_0)_{zzpo}^{ZZPO} (W^{\mathcal{R}})_{opqs}^{OPQS} \bar{X}_{sqtt}^{SQTT} \right] (\tilde{\chi}^{-1})^{TR} \quad .\end{aligned} \tag{43}$$

Eq. (41) and Eq. (43) constitute the main theoretical result of this work. Note the close resemblance of these expressions with Eq. (38) (corresponding to Eq. (A24) of Ref. [1]) and Eq. (A31) of Ref. [1], respectively. The important difference is that Eqs. (A24) and (A31) of Himmetoglu *et al.* [1] describe how the bare interaction is screened via the coarse graining of the susceptibility tensors. In contrast, our formulation reveals how such a coarse-graining process can introduce additional screening beyond that already captured by cRPA.

To make this last point more explicit, we can consider only the local components, $U_{\mathrm{LRT}}^{I} := U_{\mathrm{LRT}}^{II}$, substitute the average local interaction in cRPA $\langle\langle W^{\mathcal{R}} \rangle\rangle^{IIII} = U_{cRPA}^{I}$, using definition of $U_{\mathrm{cRPA}}^{I}$ given in Eq. (4) of the main text, and condense the additional terms on the right hand side of Eq. (43) in a single term $\Delta U^{I}$. This leads to the compact expression:

$$U_{\mathrm{LRT}}^{I} = U_{\mathrm{cRPA}}^{I} + \Delta U^{I} \quad . \tag{44}$$

This means that, if one neglects the exchange-correlation part of the kernel, $U_{\mathrm{LRT}}$ in its common implementation corresponds to the orbitally averaged $W^{\mathcal{R}}$ obtained by cRPA plus additional screening terms. The additional screening corresponds to components of the susceptibility that are not purely bi-diagonal, and encodes on-site exchange terms as well as the screening operated by inter-site and inter-orbital transitions happening within the $\mathcal{D}$ subspace.

## II. DENSITY-FUNCTIONAL PERTURBATION THEORY WITH MAXIMALLY LOCALIZED WANNIER FUNCTIONS AS HUBBARD PROJECTORS

In this section we briefly describe the extension of density-functional perturbation theory (DFPT) [7, 8] to the case of Hubbard projectors built using maximally-localized Wannier functions (MLWFs). For the sake of simplicity the formalism is presented here for insulating materials, using norm-conserving pseudopotentials, and the spin-unpolarized case.

First, we employ the recently developed interface between the DFT+$U$ implementation in Quantum ESPRESSO and the Wannier90 code, called wannier2pw, which enables the use of MLWFs as Hubbard projectors for ground-state DFT+$U$ calculations [9]. Next, we aim to extend the HP code [10] of Quantum ESPRESSO - originally designed for computing Hubbard parameters based on DFPT in the basis of (orthogonalized) atomic orbitals - to the case where MLWFs are used as Hubbard projectors. The core DFPT framework remains largely unchanged from the original formulations [7, 8]; only the definition of the response occupation matrices must be revised to incorporate MLWFs as projector functions. The details of this generalization are presented below.

By representing the atomic site indices as $I = (l, s)$ and $J = (l', s')$, where $l$ and $l'$ are the Bravais lattice indices, while $s$ and $s'$ are the atomic site indices inside the unit cells, we can write the self-consistent (interacting) response matrices $\tilde{\chi}^{IJ}$ as [7]: $\tilde{\chi}^{sl,s'l'} = \sum_m dn^{sl}_{mm}/d\lambda^{s'l'}$, where $m$ is the magnetic quantum number associated with a user-specified Hubbard manifold with a certain orbital quantum number. Here, $n^{sl}_{mm'}$ is the on-site atomic occupation matrix, and $\lambda^{s'l'}$ is the strength of the perturbation of electronic occupations. A similar expression is used for the bare response matrices $\tilde{\chi}_0$. By following Ref. [7], the response occupation matrices can be expressed as:

$$\frac{dn^{sl}_{mm'}}{d\lambda^{s'l'}} = \frac{1}{N_{\mathbf{q}}} \sum_{\mathbf{q}}^{N_{\mathbf{q}}} e^{i\mathbf{q}\cdot(\mathbf{R}_l - \mathbf{R}_{l'})}\, \Delta^{s'}_{\mathbf{q}} n^{s}_{mm'}\,, \tag{45}$$

where $\mathbf{R}_l$ and $\mathbf{R}_{l'}$ are the Bravais lattice vectors of the $l$-th and $l'$-th primitive unit cells, respectively, and $\Delta^{s'}_{\mathbf{q}} n^{s}_{mm'}$ is the lattice-periodic part of the response atomic occupation matrix to a monochromatic perturbation of wave vector $\mathbf{q}$ [7]:

$$\Delta^{s'}_{\mathbf{q}} n^{s}_{mm'} = \frac{1}{N_{\mathbf{k}}} \sum_{\mathbf{k}}^{N_{\mathbf{k}}} \sum_{n}^{N_{\text{occ}}} \Big[ \langle u_{n,\mathbf{k}} | \phi^{s}_{m',\mathbf{k}} \rangle \langle \phi^{s}_{m,\mathbf{k}+\mathbf{q}} | \Delta^{s'}_{\mathbf{q}} u_{n,\mathbf{k}} \rangle + \langle u_{n,\mathbf{k}} | \phi^{s}_{m,\mathbf{k}} \rangle \langle \phi^{s}_{m',\mathbf{k}+\mathbf{q}} | \Delta^{s'}_{\mathbf{q}} u_{n,\mathbf{k}} \rangle \Big]\,. \tag{46}$$

Here we used the fact that KS wavefunctions are Bloch functions, $\psi_{n,\mathbf{k}}(\mathbf{r}) = (1/\sqrt{N_{\mathbf{k}}})\, e^{i\mathbf{k}\cdot\mathbf{r}}\, u_{n,\mathbf{k}}(\mathbf{r})$, and the response KS wavefunctions are similarly expressed as $\Delta^{s'}_{\mathbf{q}} \psi_{n,\mathbf{k}}(\mathbf{r}) = (1/\sqrt{N_{\mathbf{k}}})\, e^{i(\mathbf{k}+\mathbf{q})\cdot\mathbf{r}}\, \Delta^{s'}_{\mathbf{q}} u_{n,\mathbf{k}}(\mathbf{r})$ [7], where $u_{n,\mathbf{k}}(\mathbf{r})$ and $\Delta^{s'}_{\mathbf{q}} u_{n,\mathbf{k}}(\mathbf{r})$ are the lattice-periodic parts of the ground-state and response KS wavefunctions, respectively. On the other hand, $\phi^{s}_{m,\mathbf{k}}(\mathbf{r})$ are the lattice-periodic parts of the Bloch sums of the localized functions $\phi^{s}_{m}(\mathbf{r} - \mathbf{R}_l)$, namely $\phi^{s}_{m,\mathbf{k}} = \sum_{\mathbf{R}_l} e^{-i\mathbf{k}\cdot(\mathbf{r}-\mathbf{R}_l)} \phi^{s}_{m}(\mathbf{r} - \mathbf{R}_l)$ [7]. Next, $N_{\text{occ}}$ is the number of occupied KS states in the primitive unit cell, while $N_{\mathbf{k}}$ and $N_{\mathbf{q}}$ is the number of $\mathbf{k}$ and $\mathbf{q}$ points in the Brillouin zone, respectively. Equation (46) shows that the quantities $\Delta^{s'}_{\mathbf{q}} n^{s}_{mm'}$ can be computed by knowing $\Delta^{s'}_{\mathbf{q}} u_{n,\mathbf{k}}(\mathbf{r})$. Since the perturbative problem is expanded to first order, perturbations at different wavelengths do not interact with each other, and it can be shown that the responses $\Delta^{s'}_{\mathbf{q}} u_{n,\mathbf{k}}(\mathbf{r})$ can be obtained directly from the self-consistent solution of the Sternheimer equation specialized to single lattice-periodic $\mathbf{q}$-specific (i.e. monochromatic) perturbations [7]. Further details about the DFPT formalism can be found in the original paper [7]. Here, instead, we focus on the extension of DFPT to the case when the localized functions $\phi^{s}_{m}(\mathbf{r} - \mathbf{R}_l)$ are chosen to be MLWFs computed using the Wannier90 code [11].

The main challenge when using MLWFs within the DFPT framework is that the lattice-periodic parts of the Bloch sums of MLWFs at $\mathbf{k}+\mathbf{q}$ points, $\phi^{s}_{m,\mathbf{k}+\mathbf{q}}(\mathbf{r})$, are not directly available. The Wannierization is performed on top of the DFT+$U$ ground state calculated using the original $\mathbf{k}$ point grid, which does not provide information for the shifted $\mathbf{k}+\mathbf{q}$ points. Performing a separate Wannierization on a grid shifted by $\mathbf{q}$ is not a viable solution because the Bloch sums at $\mathbf{k}$ and $\mathbf{k}+\mathbf{q}$ must originate from the same Wannierization procedure. Otherwise, uncontrolled phase factors could be introduced during operations such as diagonalization, potentially affecting the results. To address this issue, we follow the strategy proposed in Ref. [12]. The key idea is to exploit the mapping $\mathbf{k}+\mathbf{q} = \mathbf{k}' + \mathbf{G}$, where the $\mathbf{k}+\mathbf{q}$ point is mapped onto another $\mathbf{k}'$ point within the original grid, modulo a reciprocal lattice vector $\mathbf{G}$. As a result, we can write:

$$\phi^{s}_{m,\mathbf{k}+\mathbf{q}}(\mathbf{r}) = e^{-i\mathbf{G}\cdot\mathbf{r}} \phi^{s}_{m,\mathbf{k}'}(\mathbf{r})\,. \tag{47}$$

However, this mapping approach requires that the $\mathbf{q}$ point grid is commensurate with the $\mathbf{k}$ point grid.

## III. COMPUTATIONAL DETAILS

We perform all DFT calculations using Quantum ESPRESSO v6.6 [13, 14] using the Perdew-Burke-Ernzerhof (PBE) [15] exchange-correlation functional together with norm-conserving pseudopotentials from the PseudoDojo library [16]. All calculations are performed for the spin-unpolarized case. We use a kinetic-energy cutoff for the KS wavefunctions of 84 Ry for $KCuF_3$ and 85 Ry for $Sr_2FeO_4$, and four times larger cutoffs for the charge density, respectively. Both cubic $KCuF_3$ and tetragonal $Sr_2FeO_4$ are fully relaxed including the cell parameters before proceeding with the calculations of Hubbard parameters. We use the "cold" smearing method [17] with a broadening parameter of 0.01 Ry. To construct the Hubbard projectors, we use MLWFs obtained using the Wannier90 code v3.1 [11, 18], and we converge the sum of the spreads of the MLWFs to $10^{-9}$ Å$^2$.

To perform LRT calculations using MLWFs as Hubbard projectors, we build upon our previous implementation of the interface between DFT+$U$ and Wannier90 [9], and here we extend DFPT formalism [7, 10] for computing Hubbard $U$ to the use of MLWFs (see Sec. II). The motivation to use DFPT with primitive cells instead of the original LRT supercell approach comes from the much reduced computational cost [10], while the numerical values of the Hubbard parameters between these two approaches are identical modulo the numerical noise [7, 10]. This extended formalism is implemented in the custom version of the HP code (`hp.x` executable) [10] of the Quantum ESPRESSO distribution.

The convergence precision of the DFPT calculations depends on the density of the $\mathbf{q}$ point grid [10], which encodes the size of the supercell of the LRT approach when computing the $\tilde{\chi}$ and $\tilde{\chi}_0$ response matrices. Currently, our implementation is limited to $\mathbf{q}$ point grids that are commensurate with the $\mathbf{k}$ point grid that is used for the ground-state DFT(+$U$) calculation (see Sec. II). Due to this, the LRT results for $KCuF_3$ are obtained with a $8 \times 8 \times 8$ $\mathbf{k}$ point grid and a $4 \times 4 \times 4$ $\mathbf{q}$ point grid, while for $Sr_2FeO_4$ we use a $6 \times 6 \times 6$ $\mathbf{k}$ point grid and a $3 \times 3 \times 3$ $\mathbf{q}$ point grid. Due to technical limitations (the current implementation of DFPT calculation of $U$ with Wannier function does not exploit symmetry), we performed convergence tests using Löwdin-orthonormalized atomic orbitals as Hubbard projectors. From these tests, we estimate that the $U_{\mathrm{LRT}}$ values reported in this work are accurate to about 0.1 eV (and tend to underestimate the fully converged value by approximately this amount).

For our cRPA calculations we employ the RESPACK code (v. 20201117) [19] using the wan2respack interface for Quantum ESPRESSO and Wannier90 [20]. Results for $KCuF_3$ are converged using a $10 \times 10 \times 10$ $\mathbf{k}$ point grid, while for $Sr_2FeO_4$ we used a $7 \times 7 \times 7$ $\mathbf{k}$ point grid, employing in both cases a susceptibility cutoff of 30 Ry.

The input files containing all parameters of our calculations will be available on the Materials Cloud archive [21].


[1] B. Himmetoglu, A. Floris, S. de Gironcoli, and M. Cococcioni, International Journal of Quantum Chemistry **114**, 14 (2013).
[2] M. Cococcioni and S. de Gironcoli, Physical Review B **71**, 035105 (2005).
[3] S. Baroni, S. de Gironcoli, A. Dal Corso, and P. Giannozzi, Reviews of Modern Physics **73**, 515 (2001).
[4] R. M. Martin, L. Reining, and D. M. Ceperley, *Interacting Electrons: Theory and Computational Approaches* (Cambridge University Press, Cambridge, 2016), ISBN 978-0-521-87150-1.
[5] F. Aryasetiawan, M. Imada, A. Georges, G. Kotliar, S. Biermann, and A. I. Lichtenstein, Physical Review B **70**, 195104 (2004).
[6] F. Aryasetiawan, K. Karlsson, O. Jepsen, and U. Schönberger, Physical Review B **74**, 125106 (2006).
[7] I. Timrov, N. Marzari, and M. Cococcioni, Physical Review B **98**, 085127 (2018).
[8] I. Timrov, N. Marzari, and M. Cococcioni, Physical Review B **103**, 045141 (2021).
[9] A. Carta, I. Timrov, P. Mlkvik, A. Hampel, and C. Ederer, *Explicit demonstration of the equivalence between DFT+U and the Hartree-Fock limit of DFT+DMFT* (2024), 2411.03937.
[10] I. Timrov, N. Marzari, and M. Cococcioni, Computer Physics Communications **279**, 108455 (2022), ISSN 0010-4655.
[11] G. Pizzi, V. Vitale, R. Arita, S. Blügel, F. Freimuth, G. Géranton, M. Gibertini, D. Gresch, C. Johnson, T. Koretsune, et al., Journal of Physics: Condensed Matter **32**, 165902 (2020), ISSN 0953-8984.
[12] N. Colonna, R. De Gennaro, E. Linscott, and N. Marzari, J. Chem. Theor. Comput. **18**, 5435 (2022).
[13] P. Giannozzi, S. Baroni, N. Bonini, M. Calandra, R. Car, C. Cavazzoni, D. Ceresoli, G. L. Chiarotti, M. Cococcioni, I. Dabo, et al., Journal of Physics: Condensed Matter **21**, 395502 (2009).
[14] P. Giannozzi, O. Andreussi, T. Brumme, O. Bunau, M. B. Nardelli, M. Calandra, R. Car, C. Cavazzoni, D. Ceresoli, M. Cococcioni, et al., Journal of Physics: Condensed Matter **29**, 465901 (2017), ISSN 0953-8984.
[15] J. P. Perdew, K. Burke, and M. Ernzerhof, Physical Review Letters **77**, 3865 (1996).
[16] M. J. van Setten, M. Giantomassi, E. Bousquet, M. J. Verstraete, D. R. Hamann, X. Gonze, and G. M. Rignanese, Computer Physics Communications **226**, 39 (2018), ISSN 0010-4655.
[17] N. Marzari, D. Vanderbilt, A. De Vita, and M. C. Payne, Physical Review Letters **82**, 3296 (1999).
[18] N. Marzari, A. A. Mostofi, J. R. Yates, I. Souza, and D. Vanderbilt, Reviews of Modern Physics **84**, 1419 (2012).

[19] K. Nakamura, Y. Yoshimoto, Y. Nomura, T. Tadano, M. Kawamura, T. Kosugi, K. Yoshimi, T. Misawa, and Y. Motoyama, Computer Physics Communications **261**, 107781 (2021), ISSN 0010-4655.

[20] K. Kurita, T. Misawa, K. Yoshimi, K. Ido, and T. Koretsune, Computer Physics Communications **292**, 108854 (2023), ISSN 0010-4655.

[21] A. Carta, I. Timrov, S. Beck, , and C. Ederer, *Bridging constrained random-phase approximation and linear response theory for computing Hubbard parameters*, Materials Cloud Archive (2025), to be published.
